# Supplementary material for: AI and Collective Decisions: Strengthening Legitimacy and Losers' Consent
Source: arXiv:2604.05368 source file (2026-04-07)
Supplement: Supplementary file 1 [file concept_explanations_table.tex]

\begin{table}[ht]
\footnotesize
\centering
\begin{tabular}{llp{8cm}}
\toprule
Domain & Concept & Description \\
\midrule
\multirow{4}{*}{Process Legitimacy} 
  & Understood Decisions & Did the participant understand how the decisions were made? \\
  & Trust & Did the participant trust the decisions accurately reflected the participants' views? \\
  & Adherence & Would the participant be willing to abide by the decisions? \\
  & Felt Heard & Did the participant feel their input was valuable? \\
\midrule
\multirow{11}{*}{Social Cohesion} 
  & Learning about others & Did the participant understand others' beliefs and experiences? \\
  & Feel Connected & How connected did the participant feel to others? \\
  & Respect & Did the participant respect others' beliefs and views? \\
  & Rational & Did the participant feel others were rational? \\
  & Inclusion of Self in Others  & A visual scale that estimates how close participants feel to others. \\
  & Perspective-taking & Could the participant understand how others may view the proposals? \\
  & Commonalities & Did the participant have commonalities with other participants? \\
  & Respect Pluralism & Did the participant think it's important to respect a diversity of views? \\
  & Curious About Others  & How curious was the participant about others? \\
  & Willing to Interact & Would the participant be willing to interact with others? \\
\midrule
\multirow{4}{*}{Stances and Learning} 
  & Learning about topics & Did the participant learn more about the topics? \\
  & Change stance & Did the participant report that their stance had shifted? \\
  & Topic stance & How much did the participant agree with the proposal? \\
  & Stance certainty & How certain was the participant in their stance? \\
\bottomrule
\end{tabular}
\caption{We show the hierarchy of our measurement framework here with a short description of each concept.}
\label{tab:domain_conc}
\end{table}
