# Supplementary material for: AI and Collective Decisions: Strengthening Legitimacy and Losers' Consent
Source: arXiv:2604.05368 source file (2026-04-07)
Supplement: Supplementary file 7 [file treatments.tex]

\begin{table}[h!]
\centering
\begin{tabular}{clc}
\toprule
\textbf{Condition} & \textbf{Description} & \textbf{n} \\
\midrule
A & Took AI interview \textbf{AND} saw voting visualization & 42 \\
B & Took AI interview but did \textbf{NOT} see voting visualization & 48 \\
C & No AI interview but saw voting visualization & 44 \\
D & No AI interview and did \textbf{NOT} see voting visualization & 47 \\
\bottomrule
\end{tabular}
\caption{Treatment groups, descriptions, and participant counts.}
\label{tab:treatment_groups}
\end{table}
